# Supplementary material for: Multi-State Formulation of the Frozen-Density Embedding Quasi-Diabatization Approach
Source: arXiv:2109.01877 ancillary file (2021-09-04)
Supplement: Supplementary file 1 [file supplementary_material.pdf]

# – Supporting Information –

## Multi-State Formulation of the Frozen-Density Embedding Quasi-Diabatization Approach

Patrick Eschenbach[‖], Denis G. Artiukhin[†1], and Johannes Neugebauer[‖2]

[‖] Theoretische Organische Chemie, Organisch-Chemisches Institut and Center for Multiscale Theory and Simulation, Westfälische Wilhelms-Universität Münster, Corrensstraße 40, 48149 Münster, Germany

[†] Department of Chemistry, Aarhus Universitet, DK-8000 Aarhus, Denmark

Date: September 4, 2021

[1]Email: artiukhin@chem.au.dk

[2]Email: j.neugebauer@uni-muenster.de

# S1 Implementation Details

## S1.1 Overlap and Pseudo Inverse Matrix

As mentioned in theory section of the main text (see Sec. 2) the idea of FDE-diab lay in the construction of adiabatic wave functions from $n$ quasi-diabatic states consisting of $M$ subsystems. The obtained quasi-diabatic states $\Phi_i$ are characterized by MO coefficient matrices $\mathbf{C}^{(i),\sigma}$ that are block-diagonal, if monomer basis sets are used, and contain coefficients of subsystem $I$ within blocks $\mathbf{C}_I^{(i),\sigma}$,

$$\mathbf{C}^{(i),\sigma} = \begin{pmatrix} \mathbf{C}_A^{(i),\sigma} & \mathbf{0} & \cdots \\ \mathbf{0} & \mathbf{C}_B^{(i),\sigma} & \cdots \\ \vdots & \vdots & \ddots \end{pmatrix} . \tag{1}$$

In Eq. (1), each block is $m_I \times n_{\mathrm{occ}_I}$, where $m_I$ and $n_{\mathrm{occ}_I}$ are the numbers of basis functions and occupied MOs of subsystem $I$, respectively. For this general case an MO overlap matrix $\mathbf{S}^{(ij),\sigma}$ is constructed for each spin $\sigma \in \alpha, \beta$ and states $\Phi_i$ and $\Phi_j$ as [1]

$$\mathbf{S}^{(ij),\sigma} = \begin{pmatrix} \mathbf{S}_{A,A'}^{(ij),\sigma} & \mathbf{S}_{A,B'}^{(ij),\sigma} & \cdots \\ \mathbf{S}_{B,A'}^{(ij),\sigma} & \mathbf{S}_{B,B'}^{(ij),\sigma} & \cdots \\ \vdots & \vdots & \ddots \end{pmatrix} . \tag{2}$$

The matrix in Eq. (2) contains intra-subsystem MO overlap blocks $\mathbf{S}_{I,I'}^{(ij),\sigma}$ and inter-subsystem MO overlap blocks $\mathbf{S}_{I,J'}^{(ij),\sigma}$. Note that the primes arise from the fact that, e.g., $\mathbf{S}_{A,B'}^{(ij),\sigma}$ and $\mathbf{S}_{B,A'}^{(ij),\sigma}$ are not necessarily equivalent. The primed subsystem belongs to state $\Phi_j$, while the unprimed belongs to $\Phi_i$. This can be demonstrated by considering two quasi-diabatic states $\left|A^{+\bullet}B\right\rangle$ and $\left|AB^{+\bullet}\right\rangle$, which lead to non-equivalent off-diagonal overlap blocks $\mathbf{S}_{A^{+\bullet},B^{+\bullet}}^{(ij),\sigma}$ and $\mathbf{S}_{B,A}^{(ij),\sigma}$. In our program implementation, first an atomic orbital (AO) overlap matrix $\left(\mathbf{S}^{(ij)}\right)^{\mathrm{AO}}$ is constructed. This matrix contains inter- and intra-subsystem overlaps of basis functions $\chi_\mu^{I,(i)}$ belonging to subsystem $I$ and quasi-diabatic state $i$. For example $\left(\mathbf{S}_{I,J'}^{(ij)}\right)_{\mu\nu}^{\mathrm{AO}}$ is the overlap of two AOs corresponding to the subsystems $I$ and $J'$ within the states $i$ and $j$, respectively,

$$\left(\mathbf{S}_{I,J'}^{(ij)}\right)_{\mu\nu}^{\mathrm{AO}} = \left\langle \chi_\mu^{I,(i)} \middle| \chi_\nu^{J',(j)} \right\rangle . \tag{3}$$

To obtain the MO overlap matrix from Eq. (2), the following transformation is performed,

$$\left(\mathbf{S}_{I,J'}^{(ij),\sigma}\right)^{\mathrm{MO}} = \left(\mathbf{C}_I^{(i),\sigma}\right)^T \left(\mathbf{S}_{I,J'}^{(ij)}\right)^{\mathrm{AO}} \mathbf{C}_{J'}^{(j),\sigma} , \tag{4}$$

where $\mathbf{C}_I^{(i),\sigma}$ are matrices of subsystem coefficients from Eq. (1). The superscript MO is omitted in the following for the sake of simplicity and an MO basis is assumed for the overlap and pseudo inverse matrices. After setting up the MO overlap matrix the determinant $\det\left(\mathbf{S}^{(ij)}\right)$ is calculated. In the open-shell case, the matrix $\mathbf{S}^{(ij),\sigma}$ can be factorized into two matrices with spin components $\sigma \in \{\alpha, \beta\}$ such that its determinant is given as the product $\det\left(\mathbf{S}^{(ij)}\right) = \det\left(\mathbf{S}^{(ij),\alpha}\right) \cdot \det\left(\mathbf{S}^{(ij),\beta}\right)$. To calculate $\mathbf{S}^{(ij),\sigma}$, a bidiagonal divide and conquer singular-value decomposition (as implemented in the EIGEN3 [2] library used in SERENITY [3]) is performed where the singular values $s_k^\sigma$ and the unitary matrices $\mathbf{U}^\sigma$ and $\mathbf{V}^\sigma$ of the given matrix block are used to calculate the determinant as

$$S_{ij} = \det\left(\mathbf{S}^{(ij)}\right) = \prod_{\sigma \in \{\alpha,\beta\}} \left( \prod_k s_k^\sigma \cdot \left|\det(\mathbf{U}^\sigma)\right| \cdot \left|\det(\mathbf{V}^\sigma)\right| \right). \tag{5}$$

With these quantities at hand it is possible to calculate the Moore–Penrose pseudo inverse [4–6] of $\mathbf{S}^{(ij)}$, which is used for the construction of the transition electron density. The Moore–Penrose pseudo inverse for this case is defined by

$$\left(\mathbf{S}^{(ij),\sigma}\right)^{-1} \approx \mathbf{U}^\sigma \Omega^\sigma \left(\mathbf{V}^\sigma\right)^T, \tag{6}$$

where $\Omega^\sigma$ is a diagonal matrix of $1/s_k^\sigma$. For the singular values an absolute inversion threshold of $1.0 \times 10^{-3}$ is used by default according to Ref. [7]. Each singular value below this threshold is not inverted but set to 0. Depending on the calculation setup this threshold can be changed in the calculation input file.

## S1.2 Transition Density and Hamilton Matrix

The real-space transition-electron density $\rho^{(ij),\sigma}(\vec{r})$ is defined as a sum of products of the transition-density matrix elements $P_{\mu\nu}^{(ij),\sigma}$ and atom-centered basis functions $\chi_{\mu/\nu}(\vec{r})$,

$$\begin{aligned} \rho^{(ij),\sigma}(\vec{r}) &= \sum_{k,l}^{N_\sigma} \sum_{\mu,\nu}^{m} c_{\mu k}^{(i),\sigma} c_{\nu l}^{(j),\sigma} \left[ \left(\mathbf{S}^{(ij),\sigma}\right)^{-1} \right]_{lk} \chi_\mu(\vec{r}) \chi_\nu(\vec{r}) \\ &= \sum_{\mu,\nu}^{m} P_{\mu\nu}^{(ij),\sigma} \chi_\mu(\vec{r}) \chi_\nu(\vec{r}). \end{aligned} \tag{7}$$

The matrix elements of $\mathbf{P}^{(ij),\sigma}$ are given by

$$P_{\mu\nu}^{(ij),\sigma} = \sum_{k,l}^{N_\sigma} c_{\mu k}^{(i),\sigma} c_{\nu l}^{(j),\sigma} \left[ \left(\mathbf{S}^{(ij),\sigma}\right)^{-1} \right]_{lk}. \tag{8}$$

In our implementation $\mathbf{P}^{(ij),\sigma}$ is obtained via a product of matrices,

$$\mathbf{P}^{(ij),\sigma} = \mathbf{C}^{(i),\sigma} \left(\mathbf{S}^{(ij),\sigma}\right)^{-1} \left(\mathbf{C}^{(j),\sigma}\right)^{T}, \tag{9}$$

where $\mathbf{C}^{(i),\sigma}$ are the matrices of subsystem coefficients in Eq. (1). The product of matrices in Eq. (9) leads to a transition-density matrix, which is structured as follows,

$$\mathbf{P}^{(ij),\sigma} = \begin{pmatrix} \mathbf{C}_{A}^{(i),\sigma}\tilde{\mathbf{S}}_{A,A'}^{(ij),\sigma}\left(\mathbf{C}_{A'}^{(j),\sigma}\right)^{T} & \mathbf{C}_{A}^{(i),\sigma}\tilde{\mathbf{S}}_{A,B'}^{(ij),\sigma}\left(\mathbf{C}_{B'}^{(j),\sigma}\right)^{T} & \cdots \\ \mathbf{C}_{B}^{(i),\sigma}\tilde{\mathbf{S}}_{B,A'}^{(ij),\sigma}\left(\mathbf{C}_{A'}^{(j),\sigma}\right)^{T} & \mathbf{C}_{B}^{(i),\sigma}\tilde{\mathbf{S}}_{B,B'}^{(ij),\sigma}\left(\mathbf{C}_{B'}^{(j),\sigma}\right)^{T} & \cdots \\ \vdots & \vdots & \ddots \end{pmatrix}. \tag{10}$$

In the equation above $\tilde{\mathbf{S}}_{I,J'}^{(ij),\sigma}$ are the blocks from the pseudo inverse of the overlap matrix $\left(\mathbf{S}^{(ij),\sigma}\right)^{-1}$,

$$\left(\mathbf{S}^{(ij),\sigma}\right)^{-1} = \begin{pmatrix} \tilde{\mathbf{S}}_{A,A'}^{(ij),\sigma} & \tilde{\mathbf{S}}_{A,B'}^{(ij),\sigma} & \cdots \\ \tilde{\mathbf{S}}_{B,A'}^{(ij),\sigma} & \tilde{\mathbf{S}}_{B,B'}^{(ij),\sigma} & \cdots \\ \vdots & \vdots & \ddots \end{pmatrix}. \tag{11}$$

To remove numerical noise from the off-diagonal elements of the transition-density matrix the average of corresponding elements is taken,

$$\tilde{\mathbf{P}}^{(ij),\sigma} = \frac{1}{2}\left[\mathbf{P}^{(ij),\sigma} + \left(\mathbf{P}^{(ij),\sigma}\right)^{T}\right]. \tag{12}$$

The Hamilton matrix elements are evaluated by a KS-DFT energy functional, which is scaled by the overlap of the electronic states,

$$H_{ij} = \left\langle \Phi_i \middle| \hat{H} \middle| \Phi_j \right\rangle \approx E\left[\sum_{\mu,\nu}\left(\tilde{P}_{\mu\nu}^{(ij),\alpha} + \tilde{P}_{\mu\nu}^{(ij),\beta}\right)\chi_{\mu}(\vec{r})\chi_{\nu}(\vec{r})\right] S_{ij}, \tag{13}$$

where the transition electron density is expressed by its transition density matrix using Eq. (7).

## S1.3 Density Matrix of the Adiabatic Wave Functions

The $\sigma$-density $\rho^{\sigma}(\vec{r})[\Psi_k]$ of adiabatic wave function $\Psi_k$ is defined as the linear combination of transition-electron densities $\tilde{\rho}^{(ij),\sigma}$ [8],

$$\rho^{\sigma}(\vec{r})[\Psi_k] = \frac{\sum_{i,j}^{n} B_{i,k}B_{j,k}\tilde{\rho}^{(ij),\sigma}S_{ij}}{\sum_{i,j}^{n} B_{i,k}B_{j,k}S_{ij}}, \tag{14}$$

where $B_{i,k}$ are the linear combination coefficients and $S_{ij}$ is the overlap of the quasi-diabatic states, which is calculated according to Eq. (5). Using the definition of the transition-density matrix (see Eqs. (7) and (9)) the density matrix $\mathbf{P}_k^\sigma$ of the constructed adiabatic wave functions $\Psi_k$ can be written as,

$$\mathbf{P}_k^\sigma = \frac{\sum_{i,j}^n B_{i,k} B_{j,k} \tilde{\mathbf{P}}^{(ij),\sigma} S_{ij}}{\sum_{i,j}^n B_{i,k} B_{j,k} S_{ij}}. \tag{15}$$

$\tilde{\mathbf{P}}^{(ij),\sigma}$ in Eq. (15) is calculated according to Eq. (12).

# S2 Comparison of ADF and SERENITY

## S2.1 HAB11 Benchmark Set

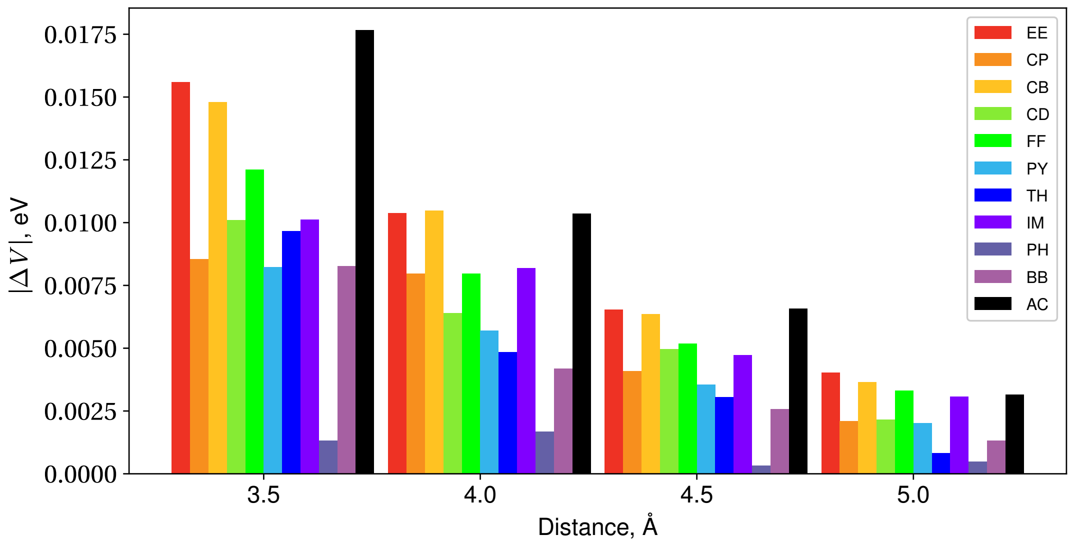


Figure S1: Absolute differences of the electronic couplings $|\Delta V|$ between SERENITY and ADF at different intermolecular distances. The molecules are labeled as follows: [EE] Ethylene Dimer, [CP] Cyclopropene Dimer, [CB] Cyclobutadiene Dimer, [CD] Cyclopentadiene Dimer, [FF] Furane Dimer, [PY] Pyrrole Dimer, [TH] Thiophene Dimer, [IM] Imidazole Dimer, [PH] Phenol Dimer, [BB] Benzene Dimer, [AC] Acetylene Dimer.

Table S1: Absolute electronic couplings $|V|$ for the HAB11 test set molecules calculated with ADF and SERENITY. The ADF results were taken from the SI of Ref. [9].

| Distance, Å | $\lvert V\rvert^{\mathrm{ADF}}$, eV | $\lvert V\rvert^{\mathrm{SERENITY}}$, eV | $\lvert\Delta V\rvert$, eV |
|---|---|---|---|
| [EE] Ethylene Dimer | | | |
| 3.50 | 0.49543 | 0.51103 | 0.01560 |
| 4.00 | 0.25655 | 0.26694 | 0.01039 |
| 4.50 | 0.13116 | 0.13769 | 0.00653 |
| 5.00 | 0.06562 | 0.06966 | 0.00404 |
| [CP] Cyclopropene Dimer | | | |
| 3.50 | 0.53267 | 0.54123 | 0.00856 |
| 4.00 | 0.24700 | 0.25497 | 0.00797 |
| 4.50 | 0.11564 | 0.11973 | 0.00409 |
| 5.00 | 0.05395 | 0.05606 | 0.00210 |
| [CB] Cyclobutadiene Dimer | | | |
| 3.50 | 0.41038 | 0.42519 | 0.01481 |
| 4.00 | 0.20849 | 0.21898 | 0.01049 |
| 4.50 | 0.10647 | 0.11284 | 0.00637 |
| 5.00 | 0.05404 | 0.05769 | 0.00365 |
| [CD] Cyclopentadiene Dimer | | | |
| 3.50 | 0.42357 | 0.43367 | 0.01010 |
| 4.00 | 0.21315 | 0.21955 | 0.00640 |
| 4.50 | 0.10627 | 0.11124 | 0.00497 |
| 5.00 | 0.05355 | 0.05571 | 0.00216 |
| [FF] Furane Dimer | | | |
| 3.50 | 0.39512 | 0.40723 | 0.01211 |
| 4.00 | 0.19403 | 0.20201 | 0.00797 |
| 4.50 | 0.09486 | 0.10004 | 0.00518 |
| 5.00 | 0.04601 | 0.04932 | 0.00332 |

Table S2: Continuation of Tab. S1.

| Distance, Å | $\lvert V\rvert^{\textsc{Adf}}$, eV | $\lvert V\rvert^{\textsc{Serenity}}$, eV | $\lvert \Delta V\rvert$, eV |
|---|---|---|---|
| [PY] Pyrrole Dimer | | | |
| 3.50 | 0.41599 | 0.42423 | 0.00824 |
| 4.00 | 0.20875 | 0.21446 | 0.00571 |
| 4.50 | 0.10498 | 0.10853 | 0.00355 |
| 5.00 | 0.05274 | 0.05477 | 0.00203 |
| [TH] Thiophene Dimer | | | |
| 3.50 | 0.41814 | 0.42780 | 0.00967 |
| 4.00 | 0.20711 | 0.21195 | 0.00484 |
| 4.50 | 0.10151 | 0.10457 | 0.00306 |
| 5.00 | 0.05014 | 0.05097 | 0.00083 |
| [IM] Imidazole Dimer | | | |
| 3.50 | 0.39050 | 0.40062 | 0.01012 |
| 4.00 | 0.19053 | 0.19873 | 0.00820 |
| 4.50 | 0.09370 | 0.09843 | 0.00473 |
| 5.00 | 0.04563 | 0.04870 | 0.00307 |
| [PH] Phenol Dimer | | | |
| 3.50 | 0.32741 | 0.32874 | 0.00133 |
| 4.00 | 0.15334 | 0.15504 | 0.00169 |
| 4.50 | 0.07285 | 0.07317 | 0.00032 |
| 5.00 | 0.03407 | 0.03455 | 0.00049 |
| [BB] Benzene Dimer | | | |
| 3.50 | 0.41392 | 0.42218 | 0.00827 |
| 4.00 | 0.20347 | 0.20766 | 0.00419 |
| 4.50 | 0.09912 | 0.10170 | 0.00258 |
| 5.00 | 0.04822 | 0.04955 | 0.00133 |
| [AC] Acetylene Dimer | | | |
| 3.50 | 0.439557 | 0.45722 | 0.01766 |
| 4.00 | 0.219702 | 0.23006 | 0.01036 |
| 4.50 | 0.107454 | 0.11403 | 0.00657 |
| 5.00 | 0.052723 | 0.05588 | 0.00315 |

## S2.2 Comparison for Molecules from Ref. [8]

### S2.2.1 Spin Populations

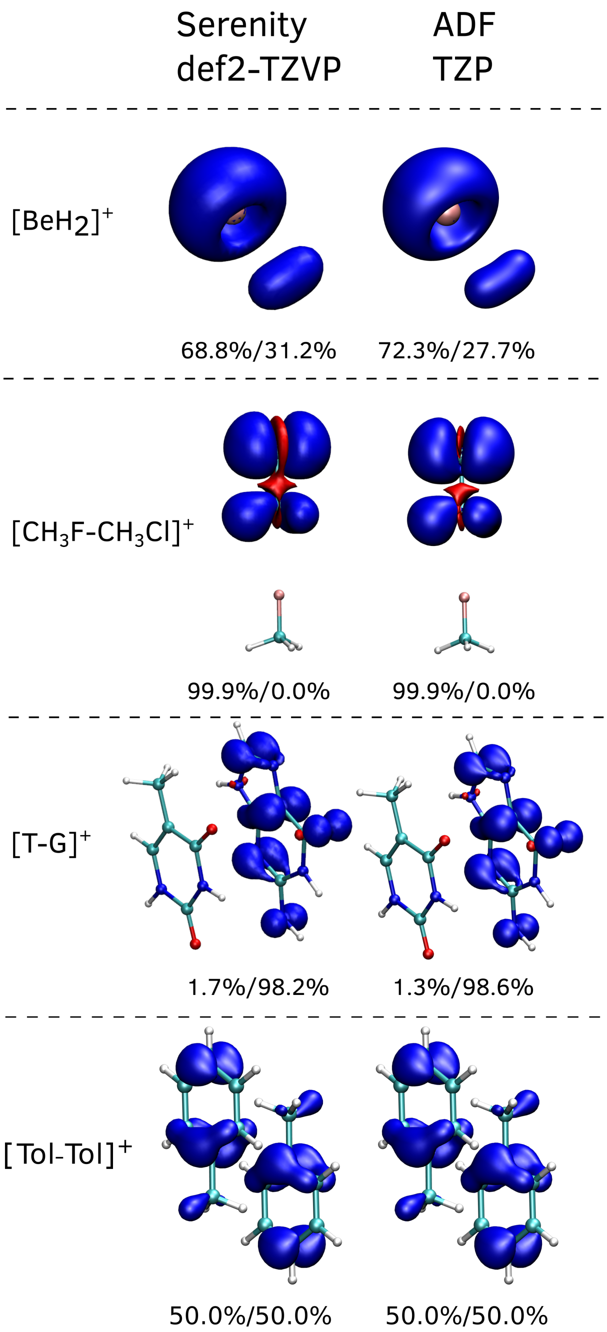


Figure S2: FDE-diab spin-density isoplots (isovalue ±0.003 a.u.) obtained with SERENITY and ADF for different radical cation complexes. Blue color corresponds to positive spin density, whereas red color corresponds to negative spin polarization. The ratios below each complex show Becke molecular spin populations.

Table S3: FDE-diab Becke atomic spin populations of the $[BeH_2]^+$ complex. In these computations, the XC functional PW91 with the kinetic-energy functional PW91k and def2-TZVP basis set were adopted. All values are given in a.u.

| Atom | ADF | SERENITY | Abs. Difference |
|---|---|---|---|
| Be | 0.72280 | 0.68779 | 0.03501 |
| H | 0.13861 | 0.15604 | 0.01743 |
| H | 0.13861 | 0.15604 | 0.01743 |

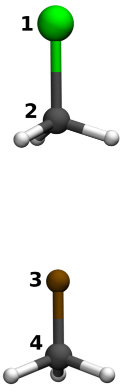


Figure S3: Atomic labels for the $[CH_3F-CH_3Cl]^+$ complex. Only heavy atoms are labeled. White, gray, green, and brown colors correspond to hydrogen, carbon, chlorine, and fluorine atoms, respectively.

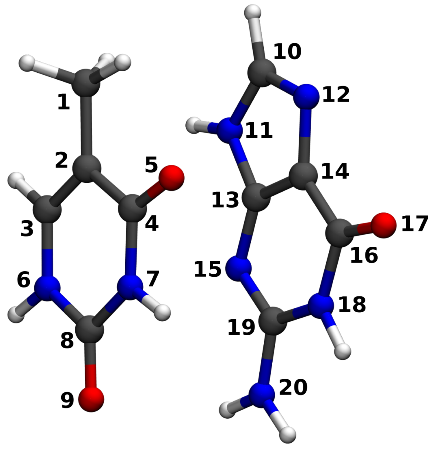


Figure S4: Atomic labels for guanine and thymine. Only heavy atoms are labeled. White, gray, red, and blue colors correspond to hydrogen, carbon, oxygen and nitrogen atoms, respectively.

Table S4: FDE-diab Becke atomic spin populations of the $[CH_3F-CH_3Cl]^+$ complex. See Fig. S3 for atomic labels. Hydrogen atoms are labeled according to the heavy atom. In these computations, the XC functional PW91 with the kinetic-energy functional PW91k and def2-TZVP basis set were adopted. All values are given in a.u.

| # | Atom | Adf | Serenity | Abs. Difference |
|---|---|---|---|---|
| 1 | Cl | 0.68568 | 0.68591 | 0.00023 |
| 2 | C | 0.03415 | 0.03234 | 0.00181 |
| $2^1$ | H | 0.16047 | 0.02300 | 0.13747 |
| $2^2$ | H | 0.05966 | 0.13934 | 0.07968 |
| $2^3$ | H | 0.05961 | 0.11861 | 0.05900 |
| 3 | F | 0.00032 | 0.00018 | 0.00014 |
| 4 | C | 0.00002 | 0.00001 | 0.00001 |
| $4^1$ | H | 0.00002 | 0.00001 | 0.00001 |
| $4^2$ | H | 0.00001 | 0.00002 | 0.00001 |
| $4^3$ | H | 0.00006 | 0.00005 | 0.00001 |

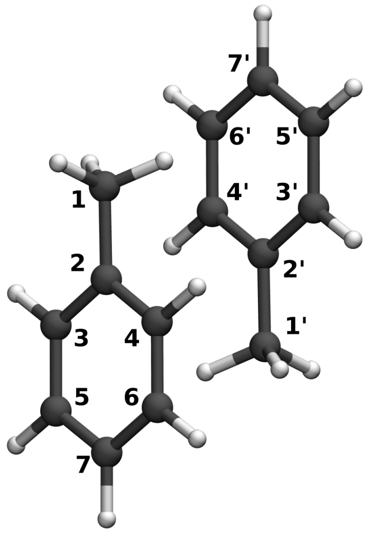


Figure S5: Atomic labels for the $[Tol-Tol]^+$ dimer. Only heavy atoms are labeled. White and gray color correspond to hydrogen and carbon atoms, respectively.

Table S5: FDE-diab Becke atomic spin populations of the $[\mathrm{T-G}]^+$ base pair. See Fig. S4 for atomic labels. Hydrogen atoms are labeled according to the heavy atom. In these computations, the XC functional PW91 with the kinetic-energy functional PW91k and def2-TZVP basis set were adopted. All values are given in a.u.

| # | Atom | Adf | Serenity | Abs. Difference |
|---|---|---|---|---|
| 1 | C | 0.00035 | 0.00033 | 0.00002 |
| $1^1$ | H | 0.00164 | 0.00203 | 0.00039 |
| $1^2$ | H | 0.00418 | 0.00412 | 0.00006 |
| $1^3$ | H | 0.00077 | 0.00047 | 0.00030 |
| 2 | C | 0.00266 | 0.00128 | 0.00138 |
| 3 | C | 0.00098 | 0.00059 | 0.00039 |
| $3^1$ | H | 0.00034 | 0.00023 | 0.00011 |
| 4 | C | 0.00039 | 0.00072 | 0.00033 |
| 5 | O | 0.00224 | 0.00161 | 0.00063 |
| 6 | N | 0.00225 | 0.00107 | 0.00118 |
| $6^1$ | H | 0.00060 | 0.00039 | 0.00021 |
| 7 | N | 0.00010 | 0.00010 | 0.00000 |
| $7^1$ | H | 0.00050 | 0.00024 | 0.00026 |
| 8 | C | 0.00000 | 0.00009 | 0.00009 |
| 9 | O | 0.00161 | 0.00078 | 0.00083 |
| 10 | C | 0.13537 | 0.13674 | 0.00137 |
| $10^1$ | H | 0.04555 | 0.04474 | 0.00081 |
| 11 | N | −0.00434 | −0.00538 | 0.00104 |
| $11^1$ | H | −0.00353 | −0.00297 | 0.00056 |
| 12 | N | 0.02186 | 0.02424 | 0.00238 |
| 13 | C | 0.08457 | 0.08401 | 0.00056 |
| 14 | C | 0.20945 | 0.20412 | 0.00533 |
| 15 | N | 0.19006 | 0.19615 | 0.00609 |
| 16 | C | −0.00938 | −0.01325 | 0.00387 |
| 17 | O | 0.17340 | 0.18177 | 0.00837 |
| 18 | N | −0.00470 | −0.00425 | 0.00045 |
| $18^1$ | H | −0.00188 | −0.00161 | 0.00027 |
| 19 | C | 0.02800 | 0.02444 | 0.00356 |
| 20 | N | 0.07285 | 0.07421 | 0.00136 |
| $20^1$ | H | 0.02057 | 0.02113 | 0.00056 |
| $20^2$ | H | 0.02375 | 0.02175 | 0.00200 |

Table S6: FDE-diab Becke atomic spin populations of the $[\mathrm{Tol{-}Tol}]^{+}$ dimer. See Fig. S5 for atomic labels of the toluene monomer. Hydrogen atoms are labeled according to the heavy atom. In these computations, the XC functional PW91 with the kinetic-energy functional PW91k and def2-TZVP basis set were adopted. All values are given in a.u.

| # | Atom | ADF | SERENITY | Abs. Difference |
|---|---|---|---|---|
| 1 | C | 0.00292 | 0.00312 | 0.00020 |
| $1^1$ | H | 0.01164 | 0.01249 | 0.00085 |
| $1^2$ | H | 0.01164 | 0.01249 | 0.00085 |
| $1^3$ | H | 0.03370 | 0.03489 | 0.00119 |
| 2 | C | 0.14309 | 0.13990 | 0.00319 |
| 3 | C | 0.04169 | 0.03901 | 0.00268 |
| $3^1$ | H | 0.01105 | 0.01092 | 0.00013 |
| 4 | C | 0.04169 | 0.03901 | 0.00268 |
| $4^1$ | H | 0.01105 | 0.01092 | 0.00013 |
| 5 | C | 0.00886 | 0.01052 | 0.00166 |
| $5^1$ | H | 0.00268 | 0.00321 | 0.00053 |
| 6 | C | 0.00886 | 0.01052 | 0.00166 |
| $6^1$ | H | 0.00268 | 0.00321 | 0.00053 |
| 7 | C | 0.12847 | 0.12916 | 0.00069 |
| $7^1$ | H | 0.04037 | 0.04033 | 0.00004 |
| $1'$ | C | 0.00292 | 0.00312 | 0.00020 |
| $1'^1$ | H | 0.03368 | 0.03489 | 0.00121 |
| $1'^2$ | H | 0.01164 | 0.01249 | 0.00085 |
| $1'^3$ | H | 0.01164 | 0.01249 | 0.00085 |
| $2'$ | C | 0.12841 | 0.12916 | 0.00075 |
| $3'$ | C | 0.04167 | 0.03901 | 0.00266 |
| $3'^1$ | H | 0.01104 | 0.01092 | 0.00012 |
| $4'$ | C | 0.04167 | 0.03901 | 0.00266 |
| $4'^1$ | H | 0.01104 | 0.01092 | 0.00012 |
| $5'$ | C | 0.00886 | 0.01052 | 0.00166 |
| $5'^1$ | H | 0.00268 | 0.00321 | 0.00053 |
| $6'$ | C | 0.00886 | 0.01052 | 0.00166 |
| $6'^1$ | H | 0.00268 | 0.00321 | 0.00053 |
| $7'$ | C | 0.14302 | 0.13990 | 0.00312 |
| $7'^1$ | H | 0.04035 | 0.04033 | 0.00002 |

# S3 DNA Base Triplets

Table S7: Molecular spin populations $P$(mol) and $\langle S^2 \rangle$ expectation values of the $[G_1AG_2]^{\bullet+}$ and $[G_1TG_2]^{\bullet+}$ radical cation complexes. In these computations, the def2-TZVP basis set was adopted.

| | $P(G_1), \%$ | $P(B), \%$ | $P(G_2), \%$ | $\langle S^2 \rangle$, a.u. |
|---|---|---|---|---|
| | | $[G_1AG_2]^{\bullet+}$ | | |
| PBE | 91.82 | 7.90 | 0.29 | 0.851 |
| B3LYP | 44.70 | 13.85 | 41.45 | 0.879 |
| CAM-B3LYP | 81.46 | 17.93 | 0.61 | 0.925 |
| B2PLYP | 92.76 | 4.29 | 2.95 | 1.072 |
| FDE-diab | 89.22 | 7.84 | 2.93 | 0.837 |
| CAS(15,16)-SCF | 97.99 | 1.43 | 0.00 | – |
| | | $[G_1TG_2]^{\bullet+}$ | | |
| PBE | – | – | – | – |
| B3LYP | 48.29 | 7.10 | 44.62 | 0.893 |
| CAM-B3LYP | 75.69 | 4.62 | 19.71 | 0.945 |
| B2PLYP | 95.22 | 2.59 | 2.22 | 1.094 |
| FDE-diab | 97.58 | 2.37 | 0.08 | 0.841 |
| CAS(15,16)-SCF | 97.47 | 2.12 | 0.00 | – |

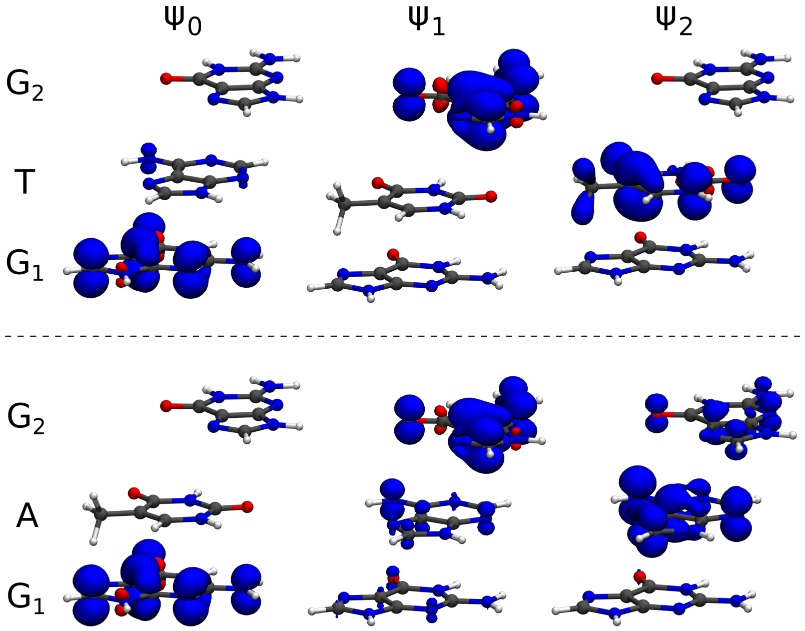


Figure S6: FDE-diab spin-density isoplots (isovalue ±0.003 a.u.) calculated for $[G_1TG_2]^{\bullet+}$ (top) and $[G_1AG_2]^{\bullet+}$ (bottom). Results are shown for the three lowest electronic states $\Psi_i$, $i = 0, 1, 2$. In these computations, the XC functional PW91 with the kinetic-energy functional PW91k and def2-TZVP basis set were adopted. Blue color indicates positive spin density, while red color shows negative spin polarization.

# S4 Benzene Stack

Table S8: Molecular spin populations calculated with different approximate FDE-diab approaches. For the FDE-diab($K, L, M$) notation, see Sec. 2.3 in the main text. All values are given in %.

| Method/Mol. index | 1 | 2 | 3 | 4 | 5 | 6 | 7 | 8 |
|---|---|---|---|---|---|---|---|---|
| FDE-diab(2,8,8) | 0.00 | 0.00 | 0.55 | 49.50 | 49.51 | 0.55 | 0.00 | 0.00 |
| FDE-diab(4,8,8) | 0.05 | 3.83 | 17.87 | 32.14 | 29.62 | 14.10 | 2.58 | 0.03 |
| FDE-diab(6,8,8) | 0.00 | 0.17 | 14.70 | 36.90 | 35.24 | 13.03 | 0.15 | 0.00 |
| FDE-diab(8,8,8) | 0.24 | 4.32 | 18.13 | 31.90 | 29.14 | 13.85 | 2.58 | 0.06 |
| FDE-diab(8,2,8) | 0.00 | 0.00 | 0.54 | 49.50 | 49.51 | 0.55 | 0.00 | 0.00 |
| FDE-diab(8,4,8) | 0.05 | 4.07 | 18.05 | 31.92 | 29.31 | 14.08 | 2.69 | 0.03 |
| FDE-diab(8,6,8) | 0.00 | 0.17 | 15.11 | 36.64 | 34.83 | 13.28 | 0.15 | 0.00 |
| FDE-diab(8,8,8) | 0.24 | 4.32 | 18.13 | 31.90 | 29.14 | 13.85 | 2.58 | 0.06 |
| FDE-diab(2,2,2) | 0.00 | 0.00 | 0.00 | 50.04 | 50.05 | 0.00 | 0.00 | 0.00 |
| FDE-diab(4,4,4) | 0.00 | 0.00 | 13.00 | 38.71 | 36.98 | 11.49 | 0.00 | 0.00 |
| FDE-diab(6,6,6) | 0.00 | 3.14 | 17.37 | 33.12 | 30.63 | 13.82 | 2.12 | 0.00 |
| FDE-diab(8,8,8) | 0.24 | 4.32 | 18.13 | 31.90 | 29.14 | 13.85 | 2.58 | 0.06 |

# References

[1] M. Pavanello, J. Neugebauer. Modelling charge transfer reactions with the frozen density embedding formalism. *J. Chem. Phys.*, **135** (2011) 234103.

[2] Gaël Guennebaud, Benoît Jacob et al. Eigen v3. http://eigen.tuxfamily.org, 2010.

[3] J. P. Unsleber, T. Dresselhaus, K. Klahr, D. Schnieders, M. Böckers, D. Barton, J. Neugebauer. SERENITY: A subsystem quantum chemistry program. *J. Comput. Chem.*, **39** (2018) 788–798.

[4] E. H. Moore. On the Reciprocal of the General Algebraic Matrix. *B. Am. Math. Soc.*, **26** (1920) 394–395.

[5] A. Bjerhammar. Rectangular reciprocal matrices, with special reference to geodetic calculations. *Bull. Geodesique*, **20**(188) (1951) 1946–1975.

[6] R. Penrose. A generalized inverse for matrices. *Math. Proc. Cambridge*, **51**(3) (1955) 406–413.

[7] P. Ramos, M. Pavanello. Quantifying Environmental Effects on the Decay of Hole Transfer Couplings in Biosystems. *J. Chem. Theory Comput.*, **10**(6) (2014) 2546–2556.

[8] D. G. Artiukhin, J. Neugebauer. Frozen-density embedding as a quasi-diabatization tool: Charge-localized states for spin-density calculations. *J. Chem. Phys.*, **148** (2018) 214104.

[9] P. Ramos, M. Papadakis, M. Pavanello. Performance of Frozen Density Embedding for Modeling Hole Transfer Reactions. *J. Phys. Chem. B*, **119** (2015) 7541–7557.
